# Supplementary material for: Ultra-compact broadband spot size converter using metamaterial cell-based inverse design
Source: arXiv:2501.06390 source file (2025-06-23)
Supplement: Supplementary file 1 [file Supporting_Information.pdf]

## Supporting Information

## Ultra-compact broadband spot size converter using metamaterial cell-based inverse design

*Alejandro Sánchez-Sánchez\*, Carlos Pérez-Armenta, José Manuel Luque-González, Alejandro Ortega-Moñux, J.Gonzalo Wangüemert-Pérez, Íñigo Molina-Fernández and Robert Halir*

## 1. Final design data

Once the 3D optimization process is complete, the following tables provide the data required to define the device according to the cell definition in Fig. 1(a) of the main text. Specifically, table S1 presents the distances for each cell of the matrix,  $d^{(i,j)}$ , while Table S2 shows the duty cycle for each cell,  $DC^{(i,j)}$ . It is important to emphasize that the dimensions of the initial taper, which adapts the input waveguide to the SWG structure, are also included. Additionally, as discussed in the main document, the matrices are symmetrical with respect to the middle row.

Table S1. Distances matrix of the final design

| $d^{(i,j)}$ [ $\mu\text{m}$ ] | Taper |       | 0     | 1     | 2     | 3     | 4     | 5     |
|-------------------------------|-------|-------|-------|-------|-------|-------|-------|-------|
| 2                             | -     | -     | 0.306 | 0.630 | 1.800 | 1.500 | 1.203 | 2.079 |
| 1                             | -     | -     | 1.234 | 1.520 | 1.188 | 0.842 | 2.342 | 1.413 |
| 0                             | 0.5   | 0.884 | 0.128 | 0.449 | 0.719 | 2.805 | 1.260 | 2.772 |
| -1                            | -     | -     | 1.234 | 1.520 | 1.188 | 0.842 | 2.342 | 1.413 |
| -2                            | -     | -     | 0.306 | 0.630 | 1.800 | 1.500 | 1.203 | 2.079 |

Table S2. Duty cycle matrix of the final design

| $DC^{(i,j)}$ [%] | Taper ( $DC_{in}$ ) |      | 1    | 2    | 3    | 4    | 5    |
|------------------|---------------------|------|------|------|------|------|------|
| 2                | -                   | -    | 31.9 | 35.8 | 36.9 | 31.9 | 47.3 |
| 1                | -                   | -    | 65.6 | 56.4 | 48.3 | 62.1 | 57.9 |
| 0                | 67.0                | 67.0 | 58.4 | 62.5 | 65.7 | 65.2 | 65.9 |
| -1               | -                   | -    | 65.6 | 56.4 | 48.3 | 62.1 | 57.9 |
| -2               | -                   | -    | 31.9 | 35.8 | 36.9 | 31.9 | 47.3 |

## 2. Input taper design

As discussed in the main text, achieving a high-performance device requires adapting the mode of the homogeneous waveguide to the SWG metamaterials used in the cell-based optimized device. The inverse design process determines the subwavelength duty cycle ( $DC_{in}$ ) and width ( $W_t$ ) that the taper must adapt to [see Fig. 1(a) in the manuscript]. Specifically, taper transitions from a homogenous silicon waveguide with a width of  $W_{in} = 500 \text{ nm}$  to a SWG waveguide with a width  $W_t = 884 \text{ nm}$  and a duty cycle of 67%, as obtained from the final 3D SWG optimization process (see tables S1 and S2).

The transition is achieved over 11 periods with  $\Lambda = 200 \text{ nm}$ , maintaining a fixed cycle while varying the segment widths. The taper follows a double linear transition: the segment of length  $a = DC \cdot \Lambda = 134 \text{ nm}$  increase linearly in width from 500 nm to 884 nm, while the segments of length  $b = (1 - DC) \cdot \Lambda = 66 \text{ nm}$  decrease linearly in width from 500 nm to 0 nm, achieving the desired SWG waveguide dimensions. The geometry of the taper can be seen in Figure S1(a) and Figure S1(b).

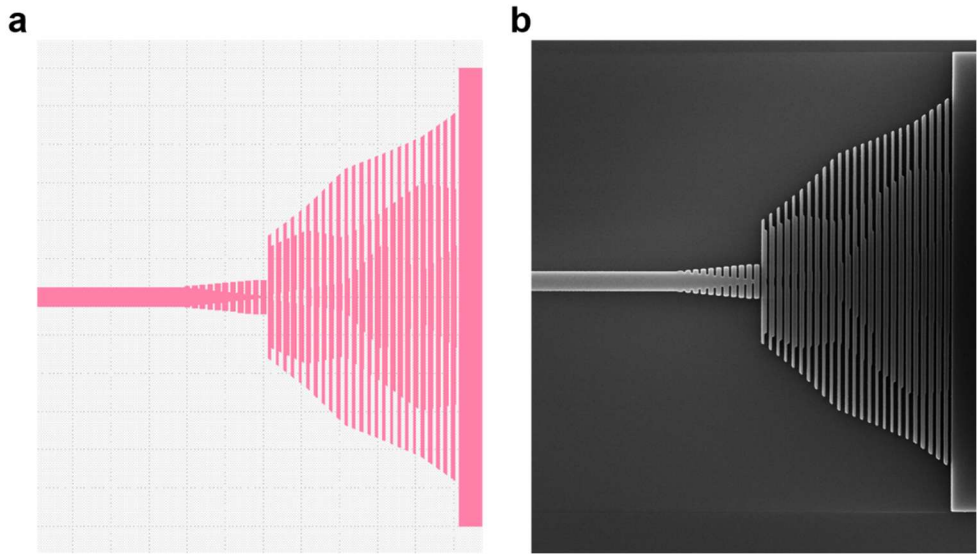

Figure S1. (a) Drawing of the final design included in the mask of fabrication. (b) Scanning electron microscope (SEM) image of the final design.

## 3. Advantage of modeling the anisotropy

In the device design, we model the anisotropy of the SWG to enhance the accuracy of the 2D homogeneous simulation. This section demonstrates the improvements achieved by introducing the anisotropic model. Figure S2(a) shows the optimization history of the score function,  $f(\mathbf{v})$ , comparing the isotropic model,  $\bar{\epsilon}^{(i,j)} = \text{diag}[\epsilon_{xx}^{(i,j)}, \epsilon_{xx}^{(i,j)}]$ , to the anisotropic model,  $\bar{\epsilon}^{(i,j)} = \text{diag}[\epsilon_{xx}^{(i,j)}, \epsilon_{zz}^{(i,j)}]$ , described in the main text. The starting points for both cases are equivalent, but the anisotropic model achieves faster improvements within just a few iterations. Moreover, the anisotropic model converges to lower losses. This behavior can be explained by the device's function as a lens. For lenses with the same maximum strength (determined by the contrast of the SWG that can be synthesized), the focal lengths is reduced when an anisotropic material is used, as demonstrated in [1].

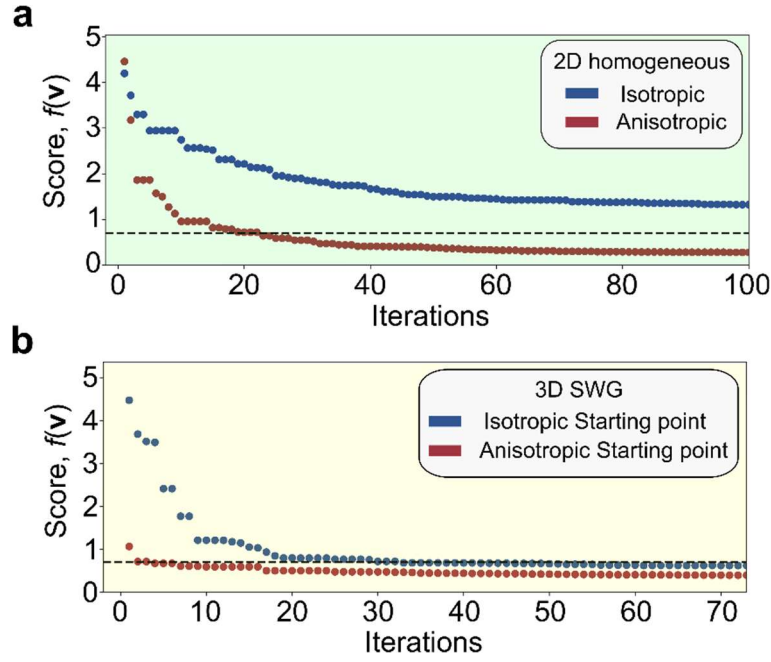

Figure S2. (a)-(b) Comparison between the optimization history of the score function,  $f(\mathbf{v})$  of the structure modeling the anisotropy versus one using an isotropic model for 2D simulation (a) and 3D simulation (b). Dashed line presents a score function of 0.7 dB in both cases.

Figure S2(b) illustrates the 3D optimization process of the devices, where the initialization corresponds to the best point obtained from Figure S2(a). It is important to note that the 3D simulation incorporates the SWG structures, where anisotropy is intrinsic. Consequently, when the best 2D candidate from the anisotropic model is used as the starting point, the initial performance is significantly better than when the starting point is provided by the isotropic model.

While the optimizer can still find a good solution starting from the best 2D candidate from the isotropic model, it requires more iterations and converges to a less optimal value. Hence, as the optimization process involves a degree of randomness and the 3D simulation are computationally expensive, incorporating the anisotropic model enhances the robustness of the optimizer, increasing the likelihood of identifying a local optimum efficiently.

#### 4. Minimizing losses of the device

To further reduce losses, one must address their origins, namely reflections, coupling to higher order modes, and radiation losses. As shown in the table below (Table S3, "original design"), in our original design these three factors contribute approximately equally to the overall losses. In the following we will use the average losses in the 1500nm to 1600nm band as figure of merit. In our original design this average loss is 0.57dB.

The main source of reflections in the original design is the interface between the end of the subwavelength structure and the beginning of the wide output waveguide. To smoothen this transition, we add the  $\sim 2\mu\text{m}$  transition shown in Table S3 ("reduced reflections"), which consists of 11 SWG periods (arrayed along the z-direction) with a pitch of 200nm and a duty-cycle of 70%, combined with nano-tapers (arrayed along the x-direction) with a pitch of 200nm, and a linearly variable duty-cycle from 30% to 70%. This yields a smooth transition while respecting a minimum feature size of 60nm. The addition of this transition yields a clear

reduction in reflections and improves the average losses to 0.34dB in the 1500nm to 1600nm band, without changing the design of original spot-size-converter.

Coupling of power to higher order modes is mainly caused by imperfections in the phase front at the end of the spot-size-converter and can thus be improved by a more sophisticated spot-size-converter. Instead of the original 5x5 sections we thus run a new optimization with 9x9 sections and furthermore include the transition at the output to reduce reflections. In this new optimization, the duty cycle of the SWG periods of the final transition is include as a variable. This results in the design shown in Table S3, "Reduced higher modes", which exhibits both reduced reflections and reduced coupling to higher order modes, especially in the 1500nm to 1600nm band, resulting in an average loss of only 0.22dB. The specific dimensions of this design are given in Table S4 and Table S5.

The remaining loss (approximately 0.22dB) is attributed mainly to the abrupt transition in waveguide width at the beginning of the spot-size-converter, which results in a small amount of radiation. Further reduction these small radiation losses has not been attempted within the scope of this work.

Table S3. Design improvements to reduce losses

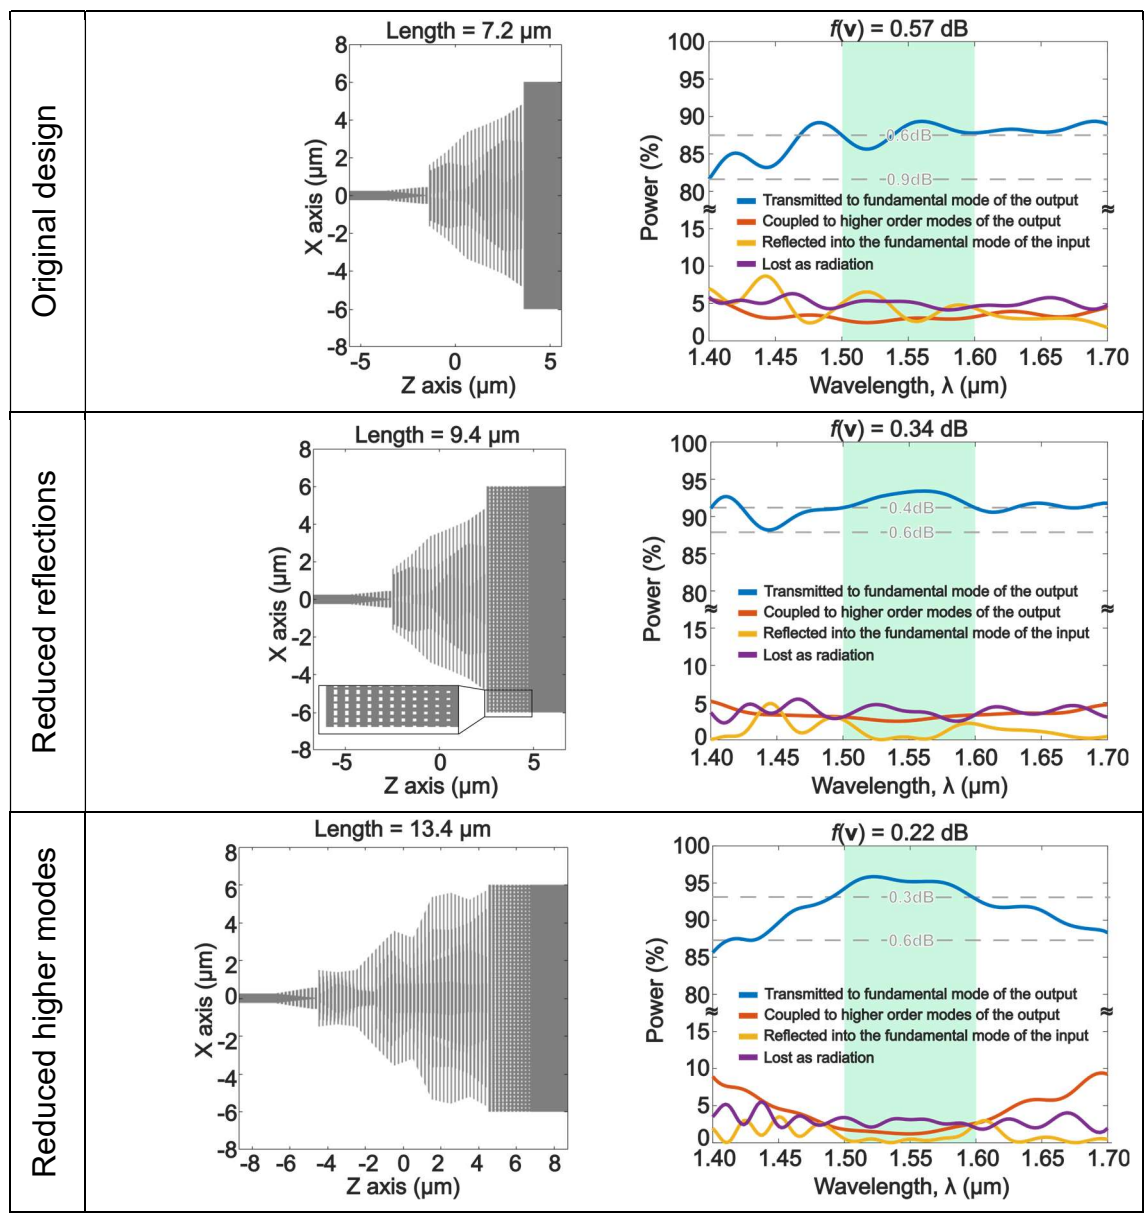

Table S4. Distances matrix of the reduced higher modes design

| $d^{(i,j)}$ [μm] | Taper in |     | 0     | 1     | 2     | 3     | 4     | 5     | 6     | 7     | 8     | 9     | Taper out |    |
|------------------|----------|-----|-------|-------|-------|-------|-------|-------|-------|-------|-------|-------|-----------|----|
| 4                | -        | -   | 0.365 | 0.128 | 0.785 | 1.013 | 0.933 | 0.944 | 1.69  | 1.963 | 1.212 | 0.950 | -         | -  |
| 3                | -        | -   | 0.411 | 0.136 | 0.138 | 0.965 | 0.313 | 0.717 | 1.530 | 0.944 | 1.056 | 1.083 | -         | -  |
| 2                | -        | -   | 0.544 | 0.307 | 0.111 | 0.217 | 0.954 | 0.638 | 0.153 | 0.383 | 0.383 | 1.568 | -         | -  |
| 1                | -        | -   | 0.113 | 0.419 | 0.080 | 0.062 | 0.580 | 0.124 | 1.189 | 1.391 | 1.828 | 1.370 | -         | -  |
| 0                | 0.5      | 1.1 | 0.124 | 0.769 | 0.761 | 0.593 | 1.568 | 1.530 | 1.572 | 1.793 | 1.447 | 1.580 | 12        | 12 |
| -1               | -        | -   | 0.113 | 0.419 | 0.080 | 0.062 | 0.580 | 0.124 | 1.189 | 1.391 | 1.828 | 1.370 | -         | -  |
| -2               | -        | -   | 0.544 | 0.307 | 0.111 | 0.217 | 0.954 | 0.638 | 0.153 | 0.383 | 0.383 | 1.568 | -         | -  |
| -3               | -        | -   | 0.411 | 0.136 | 0.138 | 0.965 | 0.313 | 0.717 | 1.530 | 0.944 | 1.056 | 1.083 | -         | -  |
| -4               | -        | -   | 0.365 | 0.128 | 0.785 | 1.013 | 0.933 | 0.944 | 1.69  | 1.963 | 1.212 | 0.950 | -         | -  |

Table S5. Duty cycle matrix of the reduced higher modes design

| DC <sup>(i,j)</sup> [%] | Taper in |      | 1    | 2    | 3    | 4    | 5    | 6    | 7     | 8     | 9    | Taper out |      |
|-------------------------|----------|------|------|------|------|------|------|------|-------|-------|------|-----------|------|
| 4                       | -        | -    | 33.7 | 37.4 | 38.2 | 38.1 | 35.3 | 38.9 | 32.4  | 35.0  | 32.1 | -         | -    |
| 3                       | -        | -    | 45.6 | 44.5 | 37.0 | 52.5 | 36.4 | 46.3 | 50.54 | 47.88 | 50.3 | -         | -    |
| 2                       | -        | -    | 54.3 | 53.7 | 41.1 | 51.6 | 51.5 | 52.2 | 41.8  | 54.7  | 52.4 | -         | -    |
| 1                       | -        | -    | 67.5 | 63.3 | 64.6 | 61.3 | 55.1 | 56.1 | 60.1  | 59.4  | 60.7 | -         | -    |
| 0                       | 63.2     | 63.2 | 65.0 | 62.8 | 69.7 | 62.3 | 65.2 | 65.4 | 68.4  | 68.5  | 66.9 | 68.4      | 68.4 |
| -1                      | -        | -    | 67.5 | 63.3 | 64.6 | 61.3 | 55.1 | 56.1 | 60.1  | 59.4  | 60.7 | -         | -    |
| -2                      | -        | -    | 54.3 | 53.7 | 41.1 | 51.6 | 51.5 | 52.2 | 41.8  | 54.7  | 52.4 | -         | -    |
| -3                      | -        | -    | 45.6 | 44.5 | 37.0 | 52.5 | 36.4 | 46.3 | 50.54 | 47.88 | 50.3 | -         | -    |
| -4                      | -        | -    | 33.7 | 37.4 | 38.2 | 38.1 | 35.3 | 38.9 | 32.4  | 35.0  | 32.1 | -         | -    |

## 5. Reflectogram characterization

Figure 5(a), reproduced below for easier reference, shows the measurement of multiple concatenated devices, which provide the data for the cutback analysis. This measurement exhibits multiple ripples, corresponding to the cavities formed due to the reflections of the spot-size convert. This section aims to clarify the origin of this ripples and to exploit them for quantifying the device reflectivity.

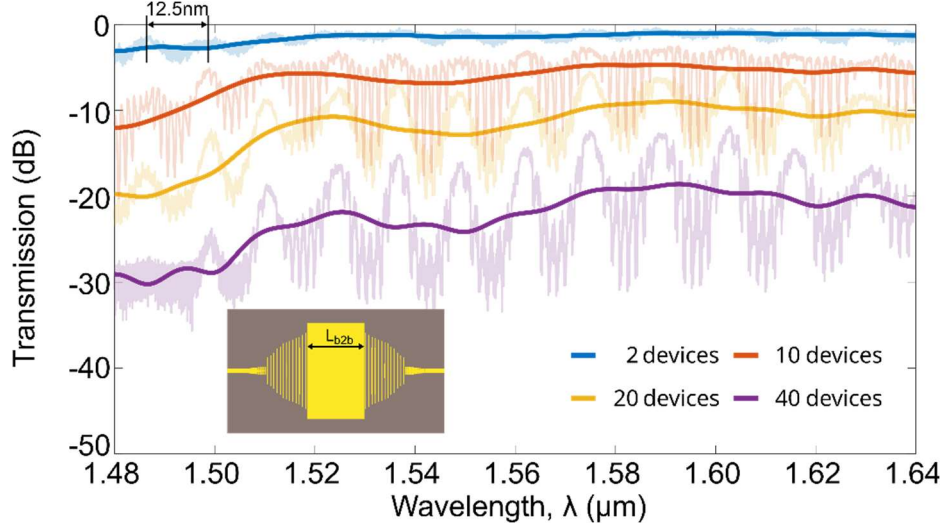

Transmission measurements of different numbers of devices in back-to-back configuration. Pale lines represent raw data, while vivid lines indicate measurements processed with a minimum phase algorithm to eliminate reflections.

The pale blue curve (labelled “2 devices”) corresponds to the transmission through a single pair of spot-size converters, and the small ripple on the transmission curve arises from the cavity formed between this pair. Indeed, the free spectral range of this ripple of  $\sim 12.5\text{nm}$ , matches well with the theoretical expression:  $\text{FSR} = \frac{\lambda_0^2}{2L_{b2b}n_g} = 12.3\text{nm}$ , for a cavity length of  $L_{b2b} = 25\mu\text{m}$ , a group index of the wide waveguide of 3.9 and a central wavelength  $\lambda_0 = 1.55\mu\text{m}$ . To further examine the reflections in this structure we use the minimum phase technique described in [2] to compute the reflectogram shown in Figure S3, which reveals a clear reflection peak at an on-chip distance corresponding to the distance between spot-size-converters. The reflection spectrum can be obtained from the reflectogram by isolating the reflection peak, Fourier transforming it, and taking the square root (because light bounces twice, once at each end of the cavity, before it reaches the output). As shown in Figure S4 below, this yields a reflection of 4% consistent with our simulation results in the Figure 2(c).

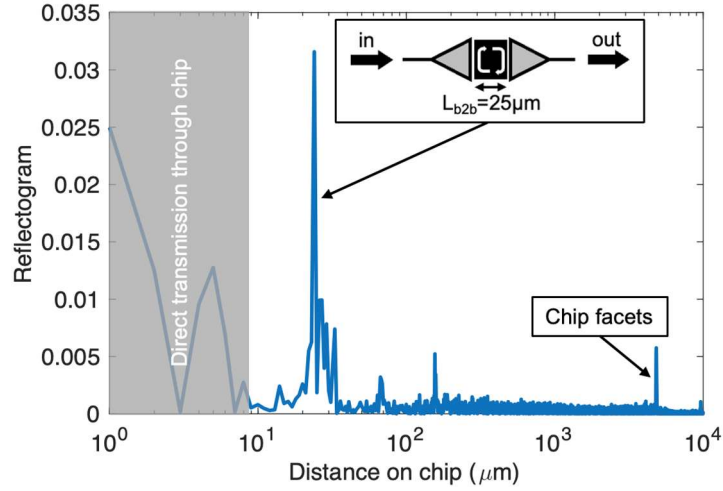

Figure S3. Reflectogram of a single back-to-back test structure (2 devices) obtained from the measurement data with minimum phase technique.

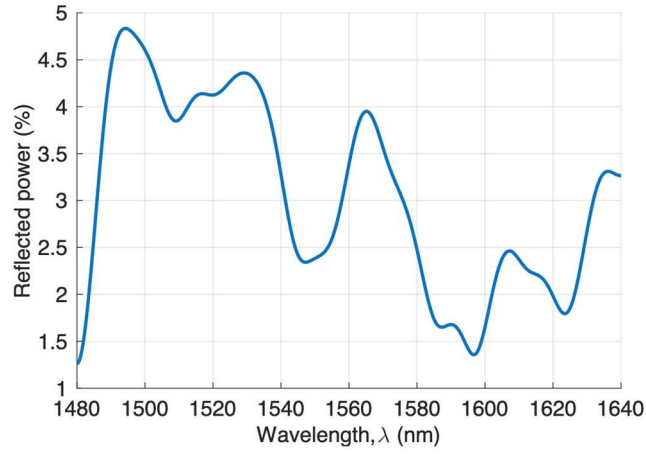

Figure S4. Reflection spectrum obtained by filtering the reflectogram.

The pale red curve (labelled “10 devices”) in Fig.5(a) corresponds to the transmission through five pairs of spot-size-converters. It exhibits two distinct ripples, one with a free spectral range of  $\sim 12.5\text{nm}$  which corresponds to the  $25\mu\text{m}$  long cavity discussed in the previous paragraph, and second one with a free spectral range of  $\sim 1.5\text{nm}$ , which corresponds to the  $200\mu\text{m}$  distance between back-to-back structures:  $\text{FSR} = \frac{\lambda_0^2}{2Ln_g} = 1.46\text{nm}$ , for a cavity length of  $L = 200\mu\text{m}$ , a group index of the single mode interconnecting waveguide of 4.1 and a central wavelength  $\lambda_0 = 1.55\mu\text{m}$ . The ripples appear much stronger than in the test structure with a single pair of spot-size-converters. While the individual reflectivity of the spot-size-converter has of course not changed, here multiple reflections form coupled cavities, producing strong interference effects. These cavities are also apparent in the reflectogram of the “10 devices” measurement shown below in Figure S5:

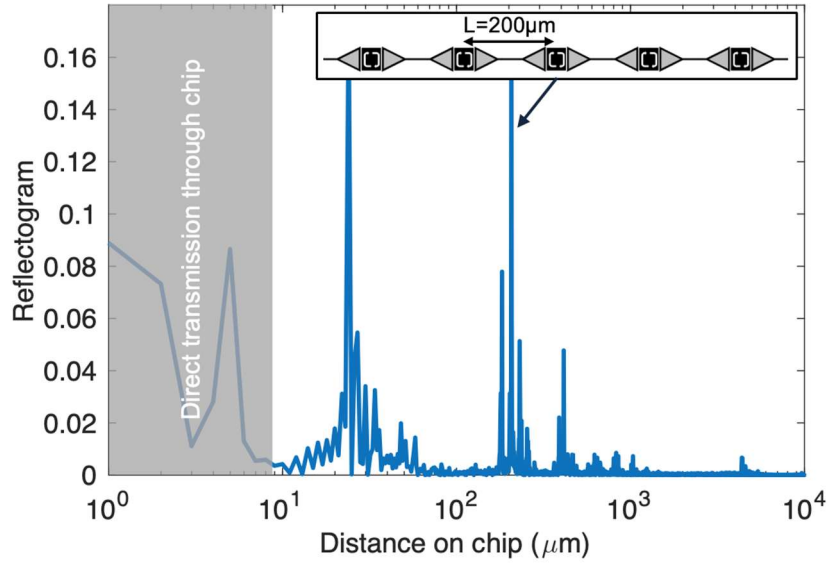

Figure S5. Reflectogram of a test structure with five back-to-back spot-size-converters (10 devices).

The curves with “20 devices” and “40 devices” exhibit similar effects.

To obtain the smooth vivid curves in Fig. 5(a) we use the minimum phase algorithm described in [2]: the direct transmission through the chip is isolated in the reflectogram and then Fourier transformed to obtain the transmission spectrum without reflections.

In order to reduce the reflectivity of the device, we have shown in the previous section that an adequate transition region between the subwavelength structure and the wide output waveguide can reduce reflections from 4.5% to below 0.9%.

## References

1. J. M. Luque-González, R. Halir, J. G. Wangüemert-Pérez, J. de-Oliva-Rubio, J. H. Schmid, P. Cheben, Í. Molina-Fernández, and A. Ortega-Moñux, *Laser & Photonics Reviews* **13**, 1900172 (2019).
2. R. Halir, Í. Molina-Fernández, J. G. Wangüemert-Pérez, A. Ortega-Moñux, J. de-Oliva-Rubio, and P. Cheben, *Opt. Express* **17**, 8349 (2009).
